# Supplementary material for: Evaluating Uncertainty-based Failure Detection for Closed-Loop LLM Planners
Source: arXiv:2406.00430 source file (2025-03-16)
Supplement: Supplementary file 1 [file appendix.tex]

\section*{APPENDIX}
